# Supplementary material for: Stochastic robustness and relative stability of multiple pathways in biological networks
Source: arXiv:1510.07784 source file (2015-10-27)
Supplement: Supplementary file 1 [file Supplementary_material_v3.pdf]

# Stochastic robustness and relative stability of multiple pathways in biological networks
# Supplementary Material

Yongyi Guo[1], Zhiyi You[1], Min Qian[1], and Hao Ge[2*]
[1]School of Mathematical Sciences, Peking University, Beijing, 100871, PRC.
[2]Beijing International Center for Mathematical Research and Biodynamic
Optical Imaging Center, Peking University, Beijing, 100871, PRC.
(Dated: October 9, 2015)

## STOCHASTIC TRAJECTORIES AND ILLUSTRATION OF TWO PHASES

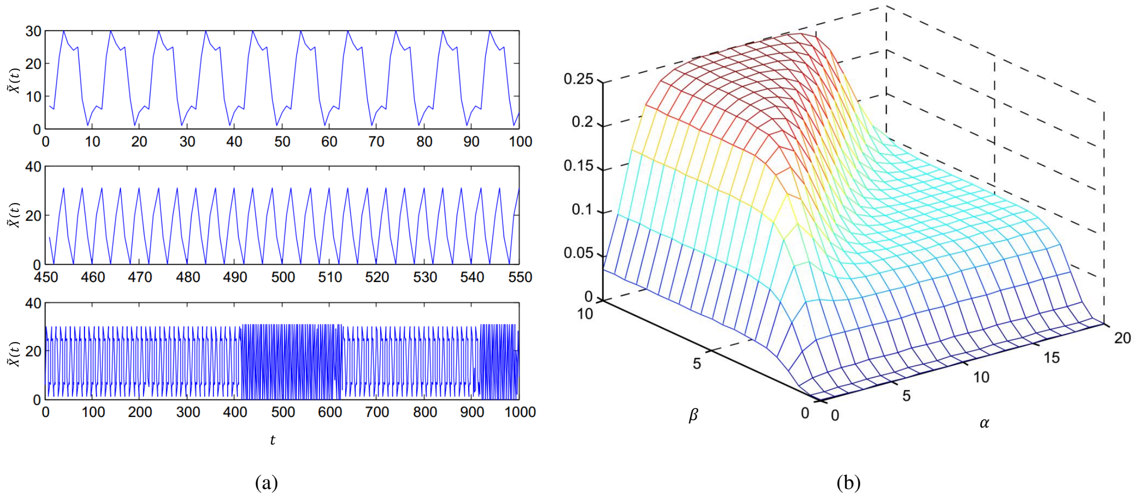


FIG. 1: Stochastic trajectory and illustration of two phases. (a) Stochastic trajectory and synchronization. Simulations are carried out with the parameters $\alpha = 8, \beta = 3$ and $\gamma = +\infty$. The x-axis ($t$) denotes time, while the y-axis $\tilde{X}(t)$ denotes the node number (0-31), derived by replacing "0" with "-1" in its binary representation $X(t)$. (b) Net flux of cycle 2 with respect to $\alpha$ and $\beta$ given $\gamma = +\infty$.

Fig. 1 (a) above directly visualizes a random trajectory when $\alpha = 8, \beta = 3$ and $\gamma = +\infty$. The upper panel reveals the phenomenon of the local rapid synchronization (cycle 1, period=10) during a very short time period. The middle panel is a later part of this random trajectory, which shows another set of synchronized dynamics (cycle 2, period=4). The lower panel shows the trajectory in a greater scale, from which we can observe its transitions between cycle 1 and cycle 2 in a somehow regular manner.

How to quantitatively characterize such a 'certain' behavior under the stochastic environment? Mathematically, the relative stability of different pathways could be described by the 'net cycle fluxes'. With calculations one can discover that, under certain restrictions of $\alpha, \beta$ and $\gamma$ there will be a fixed probability distribution between the two cycles, while in some rare occasions the net flux of cycle 1 will decrease to zero as the noise tends to zero. To visualize part of this theoretical result, Fig. 1(b) presents the net flux of cycle 2 with respect to $\alpha$ and $\beta$ given $\gamma = +\infty$, where flux = 0.25(reciprocal of its number of states) indicates its dominance, namely the "noise induced global attractive behavior". It seems evident that when $\lim_{\beta\to+\infty} \alpha/\beta$ is a nonnegative constant less than 2, this global attractive phenomenon will occur as $\beta \to +\infty$(noise intensity tends to zero).

## THEORY OF EXPONENTIALLY PERTURBED MARKOV CHAIN AND ITS APPLICATIONS TO OUR STOCHASTIC BOOLEAN NETWORK MODEL

In the main text we state an important theorem from [1] in Eq. (3):

$$\lim_{\beta\to\infty} \frac{1}{\beta} \log\langle \tau_{ij} \rangle = \Delta\Phi_{ij},$$

but the exact definition of $\Delta\Phi_{ij}$– how it's computed in practice– is not explicitly mentioned.

Generally, let us consider a family of Markov chains on a finite state space $S$ with transition probability matrices $\{\mathbb{P}^{\beta}; \beta \in [0, +\infty]\}$ satisfying

$$p^{\infty}(\xi, \eta) = \lim_{\beta \to \infty} p^{\beta}(\xi, \eta);$$

$$C_{\xi\eta} = \lim_{\beta \to \infty} -\frac{1}{\beta} \log p^{\beta}(\xi, \eta)$$

exist for any $\xi, \eta \in S$, and

$$C_{\xi\eta} > 0 \quad \text{if} \quad p^{\infty}(\xi, \eta) = 0.$$

This system is called an exponentially perturbed Markov chain, where all the $C_{\xi\eta}$ can be viewed as activation energy difference between the states $\xi$ and $\eta$. For any subset $K \subset S$, denote the exit time of the Markov chain $\{X_n\}$ out of $K$ to be

$$\mu(K) = \inf\{n; X_n \notin K\}$$

and the hitting time to $K$ be

$$\sigma(K) = \inf\{n; X_n \in K\}.$$

Assume that all the recurrent class(attractors) of $\mathbb{P}^{\infty}$ are $\{A_1, ..., A_s\}$, each $A_i$ having its "attractive basin"

$$B_i = \{\xi; P^{\infty}(\sigma(A_i) < \infty | X_0 = \xi) > 0\}.$$

The activation energy along each trajectory $\{X_i = \xi_i, i = 0, 1, 2, \cdots, l\}$ is defined to be $\sum_{k=1}^{l} C_{\xi_{k-1}\xi_k}$. Then intuitively, the minimum "activation energy barrier" for the exit from $B_i$ should be

$$T(B_i) = \min\left\{\sum_{k=1}^{l} C_{\xi_{k-1}\xi_k}; l \geqslant 1, \xi_0 \in A_i, \xi_1, ..., \xi_{l-1} \in B_i, \xi_l \notin B_i\right\},$$

and

$$\Delta\Phi_{ij} = \min\left\{\sum_{k=1}^{l} C_{\xi_{k-1}\xi_k}; l \geqslant 1, \xi_0 \in A_i, \xi_1, ..., \xi_{l-1} \in B_i, \xi_l \in B_j,\right\},$$

which characterizes the minimum activation energy barrier for transiting from the $i$-th attractor to the $j$-th one.

We then apply this general theory to our stochastic Boolean network model. First apply to the situation where the stochastic model approaches the deterministic one as $\delta = 1$. Let $S = \{0, ..., 31\}$; $A_1$ and $A_2$ be cycle 1 and 2, with corresponding $B_i$ representing their attractive basins; and $\mathbb{P}^{\beta}$ defined between states of $S$ according to Eq. (2) in the main text as $\alpha = k\beta, \gamma = l\beta$. In this case it's not difficult to check that the above system forms an exponentially perturbed Markov chain, and its limiting chain $\mathbb{P}^{\infty}$ equals our deterministic model when $\delta = 1$. Moreover with concrete expressions of transition probability we can easily cipher out the value of $C_{\xi\eta}$: if $\xi = (\xi_1, ..., \xi_5)$, $\eta = (\eta_1, ..., \eta_5)$, then

$$C_{\xi\eta} = \sum_{i=1}^{5} C_{\xi\eta}^{(i)},$$

where

$$C_{\xi\eta}^{(i)} = \begin{cases} 2|H_i| & H_i\eta_i < 0, \text{ and } \xi \neq 6 \text{ or } i \geqslant 2; \\ k & H_i = 0, \xi_i = -\eta_i, \text{ and } \xi \neq 6 \text{ or } i \geqslant 2; \\ l & \xi_i = \eta_i, \xi = 6 \text{ and } i = 1; \\ 0 & \text{otherwise}, \end{cases}$$

and

$$H_i = \sum_{j=1}^{5} T_{ij}\xi_j.$$

Particularly, $C_{\xi\eta} = 0$ if there exists an edge from $\xi$ to $\eta$ in $\mathbb{P}^{\infty}$.

Based on the above facts we deduce that

$$\Delta\Phi_{21} = 2$$

with optimal paths

$$0 \to 4, \quad 0 \to 22, \quad 0 \to 28, \quad 20 \to 27,$$
$$31 \to 3, \quad 31 \to 9, \quad 31 \to 17, \quad 11 \to 4.$$

On the other hand, if $k < 2$, then

$$\Delta\Phi_{12} = k$$

with two optimal paths

$$22 \to 31, \quad 9 \to 0;$$

while if $k \geqslant 2$ then

$$\Delta\Phi_{12} = 2$$

with optimal paths

$$1 \to 21, \quad 5 \to 23$$

and the like. Therefore, when $k < 2$, the potential well of cycle 2 will be deeper than that of cycle 1, and we may easily prove the occurrence of the global attractive behavior through further deduction in the main text by means of Eq. (3).

Similar methods can be employed as for the case of $\delta = 0$, with the differences that $A_1 = \{6\}$, and $\mathbb{P}^{\beta}$ defined according to Eq. (2) with $\alpha = k\beta, \gamma = -l\beta$. In fact, the minimum activation energy barrier of $B_1$ and the corresponding minimum paths remain the same here, but the situation in the opposite direction varies. If $k + l < 2$ then

$$\Delta\Phi_{12} = k + l$$

with two optimal paths

$$6 \to 22 \to 31,$$
$$6 \to 22 \to 30 \to 26 \to 24 \to 25 \to 9 \to 0;$$

while if $k + l \geqslant 2$ then

$$\Delta\Phi_{12} = 2$$

with at least one optimal path

$$6 \to 2.$$

Therefore, when $k + l < 2$, the potential well of cycle 2 will again be deeper than that of cycle 1, and from Eq. (3) we can prove the global attractive behavior in this case.

## A PROOF OF EQ. 4 IN THE MAIN TEXT

As is stated in the main text, the above theorem cannot explain the non-global-attractive behavior. Thus we would like to provide here a simple proof of Eq. (4), and show how to apply it to the calculations of cycle fluxes under specific parameter settings. The ideas again come from [1].

For any subset $K \subset S$ and transition probability matrix $\mathbb{P}$, denote $G(K)$ as the set of mappings $g : K \to S$ with the property that $g$ maps no nonempty subset of $K$ into itself. For $p \in K$ and $q \in S \setminus K$, we say that "$g \in G(K)$ leads $p$ to $q$" if there exist distinct states $x_1, ..., x_k$ in $K$ such that

$$g(p) = x_1, g(x_k) = q, \text{ and } g(x_j) = x_{j+1} (1 \leqslant j \leqslant k - 1),$$

and further define $G_{pq}(K)$ to be the subset of $g \in G(K)$ that leads $p$ to $q$. We also denote (for any $g : K \to S$)

$$\pi(g) = \prod_{x \in K} p(x, g(x))$$

and particularly in our case

$$\pi^\beta(g) = \prod_{x \in K} p^\beta(x, g(x)).$$

Based on above, the "potential" of the subset $K$ as well as "activation energy difference" between states can be more directly characterized in the following definitions (which accords with previous ones, see [1]):

$$T(K) = \min_{g \in G(K)} \Pi(g)$$

and

$$T_{\xi\eta}(K) = \min_{g \in G_{\xi\eta}(K)} \Pi(g),$$

where

$$\Pi(g) = \lim_{\beta \to \infty} -\frac{1}{\beta} \log \pi^\beta(g).$$

In fact we have

$$\Pi(g) = \sum_{\xi \in K} C_{\xi g(\xi)},$$
$$T(K) = \min_{g \in G(K)} \sum_{\xi \in K} C_{\xi g(\xi)}, \text{ and}$$
$$T_{\xi\eta}(K) = \min_{g \in G_{\xi\eta}(K)} \sum_{\xi \in K} C_{\xi g(\xi)}.$$

Now according to Lemma 1.3 in [1], the mean exit time satisfies

$$\mathbb{E}_p \mu(K) = \frac{\sum\limits_{g \in G(K \setminus \{p\})} \pi(g) + \sum\limits_{j \in K \setminus \{p\}} \sum\limits_{g \in G_{pj}(K \setminus \{j\})} \pi(g)}{\sum\limits_{g \in G(K)} \pi(g)}.$$

So in our model with two recurrent classes in the limiting Markov chain,

$$r^\beta \triangleq \frac{\tau_{12}}{\tau_{21}} = \frac{\mathbb{E}^\beta_{\xi_1} \mu(B_1)}{\mathbb{E}^\beta_{\xi_2} \mu(B_2)} = \frac{s_1^\beta}{s_2^\beta} \cdot \frac{\sum\limits_{g \in G(B_2)} \pi^\beta(g)}{\sum\limits_{g \in G(B_1)} \pi^\beta(g)},$$

where

$$s_1^\beta = \sum_{g \in G(B_1 \setminus \{\xi_1\})} \pi^\beta(g) + \sum_{\eta \in B_1 \setminus \{\xi_1\}} \sum_{g \in G_{\xi_1 \eta}(B_1 \setminus \{\eta\})} \pi^\beta(g)$$

and $s_2^\beta$ can be defined similarly. What we want to prove is that

$$\lim_{\beta \to \infty} s_i^\beta = |A_i|, \tag{1}$$

$$\lim_{\beta \to \infty} \frac{\sum\limits_{g \in G(B_2)} \pi^\beta(g)}{\sum\limits_{g \in G(B_1)} \pi^\beta(g)} = \frac{n_{21}}{n_{12}}. \tag{2}$$

Firstly, note that $s_1^\beta$ is the sum of a finite number of terms, each of which is a product of a finite number of probability values in $\mathbb{P}^\beta$. And since our limiting Markov chain is deterministic, for any $\eta_1, \eta_2 \in S$ we have

$$\lim_{\beta\to\infty} p^\beta(\eta_1, \eta_2) = 0 \text{ or } 1.$$

Therefore, $\lim_{\beta\to\infty} s_1^\beta$ simply equals to the number of terms in the sum that approaches 1 when $\beta \to \infty$, and more specifically, the number of $g \in G(B_1 \setminus \{\xi_1\}) \cup G_{\xi_1\eta}(B_1 \setminus \{\eta\})$ such that each "edge" $(x, g(x))$ satisfies $\lim_{\beta\to\infty} p^\beta(x, g(x)) = 1$. Apparently this happens if and only if $g$ maps every state(in its domain of definition) to its "natural successor" in the limiting deterministic model, which is implied in Fig. 2(a) and Fig. 3(a) in the main text. Here we should additionally recall that by definition $g$ cannot map any subset into itself.

If $\xi_1 \in A_1$(the limit cycle in $B_1$), there will be exactly one $g \in G(B_1 \setminus \{\xi_1\})$ satisfying the above properties, mapping each $\eta \in B_1 \setminus \{\xi_1\}$ to its natural successor in the limiting deterministic chain respectively. And there will exist $(|A_1| - 1)$ feasible states for $\eta$ such that those $g_\eta$, mapping each $\mu \in B_1 \setminus \{\eta\}$ to its natural successor, also meet the requirements of $G_{\xi_1\eta}(B_1 \setminus \{\eta\})$ – that is, $g$ not only maps no nonempty set $K \subset B_1$ into itself, but also leads $\xi_1$ to $\eta$. The set containing such states is simply $A_1 \setminus \{\xi_1\}$. In fact, it's easy to verify that $g_\eta(\eta \in A_1 \setminus \{\xi_1\})$ satisfy all our rules; however, $g_\eta(\forall\eta \in B_1 \setminus A_1)$ does not, because it maps $A_1$ into itself.

If $\xi_1 \in B_1 \setminus A_1$, there will be no $g \in G(B_1 \setminus \{\xi_1\})$ with the above properties, for the only $g$ mapping each $\eta \in B_1 \setminus \{\xi_1\}$ to its natural successor maps $A_1$ into itself. Nevertheless, there will be $|A_1|$ feasible states for $\eta$ such that $g_\eta$ defined as above meets the requirements of $G_{\xi_1\eta}(B_1 \setminus \{\eta\})$. And the set containing such states is exactly $A_1$, because if we start at $\xi_1$ in the deterministic model, we'll surely step into $A_1$; also, only if $\eta \in A_1$ can $g_\eta$ avoid mapping $A_1$ into itself.

In conclusion, whatever state $\xi_1$ is, we have $\lim_{\beta\to\infty} s_1^\beta = |A_1|$; similarly $\lim_{\beta\to\infty} s_2^\beta = |A_2|$. So in order to reach Eq. (4) in the main text we only need to prove (2).

Just like $s_i^\beta$, both the numerator and denominator in the left hand side of (2) is the sum of a finite number of terms, each of which is a product of a finite number of probability values. But there is an essential difference between this fraction and $\frac{s_1^\beta}{s_2^\beta}$: Note that $g$ cannot map any subset into itself, and there exist loops inside both $B_i$ in the deterministic model, so for any $g \in G(B_i)(i = 1, 2)$, there is at least one "edge" $(x, g(x))$ such that $g(x)$ is not the natural successor of $x$. This indicates that

$$\lim_{\beta\to\infty} \pi^\beta(g) = 0, \quad \forall g \in G(B_i),$$

and we must compare the higher order infinitesimal of the numerator and denominator.

According to Eq. (2) in the main text as well as the relation $\alpha = k\beta, \gamma = \pm l\beta$, for fixed $k$ and $l$ we can uniformly express each element of $\mathbb{P}^\beta$ as

$$p^\beta(\xi, \eta) = \prod_{i=1}^{5} \frac{1}{1 + e^{V_{\xi\eta}^{(i)}\beta}},$$

where $V_{\xi\eta}^{(i)}(\xi, \eta \in S, i \in \{1, ..., 5\})$ are some real constants. So by definition,

$$\begin{aligned} C_{\xi\eta} &= \lim_{\beta\to\infty} -\frac{1}{\beta} \log p^\beta(\xi, \eta) \\ &= \sum_{i=1}^{5} \lim_{\beta\to\infty} \log(1 + e^{V_{\xi\eta}^{(i)}\beta})/\beta \\ &= \sum_{i=1}^{5} \max\{V_{\xi\eta}^{(i)}, 0\}. \end{aligned}$$

Denote

$$\widetilde{V_{\xi\eta}^{(i)}} = \max\{V_{\xi\eta}^{(i)}, 0\},$$

then by the form of the transition probability we have

$$\begin{aligned} p^\beta(\xi, \eta) &= \prod_{i=1}^{5} e^{-\widetilde{V_{\xi\eta}^{(i)}}\beta}(1 + o(e^{-V_0\beta})) \\ &= e^{-C_{\xi\eta}\beta}(1 + o(e^{-V_0\beta})), \end{aligned}$$

where $V_0$ is some positive real number, and may depend only on $k$ and $l$.

On the other hand, we observe that for any $g \in G(B_i)$, there exist at least one path $(\xi_0, \xi_1, ..., \xi_l)$ such that $g(\xi_i) = \xi_{i+1} (0 \le i \le l-1)$; $\xi_0 \in A_i, \xi_1, ..., \xi_{l-1} \in B_i \setminus A_i$, and $\xi_l \in B_i$. (In fact if it's not the case, $g$ must have mapped at least one subset containing some elements in $A_i$ into itself.) Therefore, we have

$$\begin{aligned}\pi^\beta(g) &= \prod_{i=0}^{l-1} p^\beta(\xi_i, \xi_{i+1}) \cdot \prod_{x \in B \setminus \{\xi_0, ..., \xi_{l-1}\}} p^\beta(x, g(x)) \\ &= \prod_{i=0}^{l-1} e^{-C_{\xi_i \xi_{i+1}} \beta}(1 + o(e^{-V_0 \beta})) \cdot \prod_{x \in B \setminus \{\xi_0, ..., \xi_{l-1}\}} p^\beta(x, g(x)) \\ &= e^{-T_g \beta}(1 + o(1)) \quad (\beta \to \infty),\end{aligned}$$

where the positive constant

$$\begin{aligned}T_g &\ge \sum_{i=0}^{l-1} C_{\xi_i \xi_{i+1}} \\ &\ge \min \left\{ \sum_{k=0}^{l-1} C_{\xi_k \xi_{k+1}}; l \geqslant 1, \xi_0 \in A_i, \xi_1, ..., \xi_{l-1} \in B_i, \xi_l \notin B_i \right\} \\ &= T(B_i) = \Delta\Phi_{ij}.\end{aligned}$$

Moreover, we can see that $T_g = \Delta\Phi_{ij}$ if and only if $g$ induces one pathway from $A_i$ to the outside of $B_i$ with the least possible "energy cost", and maps the other states within its domain of definition to its natural successor in the deterministic model. (This fact guarantees that $g$ contains no loops.) Therefore, those $g$ which satisfy $T_g = \Delta\Phi_{ij}$ are in one-to-one correspondence with the pathways from $A_i$ to outside $B_i$ with the minimum energy, and

$$\sum_{g \in G(B_{1(2)})} \pi^\beta(g) \sim n_{12(21)} \Delta\Phi_{12(21)}, \quad \beta \to \infty,$$

where $n_{12}(n_{21})$ represents the number of pathways from cycle 1(2) to the attractive basin of cycle 2(1) with the least possible energy cost.

Finally, note that in non-global-attractive situations $\Delta\Phi_{12} = \Delta\Phi_{21}$, so we obtain from the above expressions that

$$\lim_{\beta \to \infty} \frac{\sum_{g \in G(B_2)} \pi^\beta(g)}{\sum_{g \in G(B_1)} \pi^\beta(g)} = \frac{n_{21}}{n_{12}},$$

which ends the proof.

To illustrate the application of Eq. (4) in the main text, we further present a simple example of computing the limiting ratio of cycle fluxes as $\alpha = k\beta, \gamma = -l\beta$ and $k + l = 2$. Here the two attractors are

$$\begin{aligned}&A_1 : 6. \\ &A_2 : 0 \to 20 \to 31 \to 11;\end{aligned}$$

By direct calculations one finds out that $\Delta\Phi_{12} = \Delta\Phi_{21} = 2$; the eight pathways from $A_2$ to $B_1$ with minimum energy cost are:

$$\begin{aligned}&0 \to 4, \quad 0 \to 22, \quad 0 \to 28, \quad 20 \to 27, \\ &31 \to 3, \quad 31 \to 9, \quad 31 \to 17, \quad 11 \to 4;\end{aligned}$$

and the three pathways from $A_1$ to $B_2$ with minimum energy cost are:

$$\begin{aligned}&6 \to 2, \\ &6 \to 22 \to 31, \\ &6 \to 22 \to 30 \to 26 \to 24 \to 25 \to 9 \to 0.\end{aligned}$$

Combining the above information and Eq. (4) gives

$$\lim_{\beta\to\infty} \frac{\tau_{12}}{\tau_{21}} = \frac{1\cdot 8}{4\cdot 3} = \frac{2}{3},$$

on the basis of which we can easily solve Eq. (5) in the main text, getting the result that

$$c_1 = \frac{2}{5}.$$

Moreover, if $k + l > 2$, the minimum energy for both sides stays the same; so do the eight optimal pathways from $A_2$ to the $B_1$. But this time only one minimum pathway remains from $A_1$ to $B_2$, which is $6 \to 2$. Therefore

$$\lim_{\beta\to\infty} \frac{\tau_{12}}{\tau_{21}} = \frac{1\cdot 8}{4\cdot 1} = 2,$$

and we deduce that

$$c_1 = \frac{2}{3}.$$

## THE IMPACT OF INTERACTION STRENGTHS ON THE MINIMUM ACTIVATION ENERGY BARRIERS

To better understand the model, it is important to identify the influence of interaction strengths between each pair of protein components – that is, elements of the matrix $T$ – on the activation energy barriers, and thus on the transition time as well as number of optimal transition paths between parallel pathways. Fortunately, as is mentioned in the main text, this goal could be achieved by our theory.

Firstly, without changing rules of their interactions, we ought to keep the sign of each entry in $T$ unaltered; and typically, we do not change the value of zero entries throughout our analysis. On the other hand, since we are primarily concerned about whether the minimum activation energy barriers are sensitive to "small" changes of $T$, we'll only elucidate situations where the absolute values of all nonzero components in $T$ vary in $(0, 2]$.

Even with the above conventions, the structure of the deterministic models may still become significantly different from their original structures in Fig. 1(b) of the main text. In fact, if we denote $T_{ij}$ as the entry in the $i$-th row and $j$-th column of $T$, then it's easy to discover that when $T_{51} + T_{54} = 0$, the above phenomenon will not happen. The reason is that in this case, for any state $\xi$, $\text{sign}(H_i)$ will remain unchanged when deciding its next state in the deterministic model (here $H_i = \sum_j T_{ij}\xi_j$, see Eq. (1) in the main text). On the contrary, however, if $T_{51} + T_{54} \neq 0$, we learn from Eq. (1) in the main text that the structure of the deterministic model surely changes. Fig. 2 (a) (b) shows the structure of the deterministic model under the condition $\delta = 1$ when $T_{51} + T_{54} > 0$ and $T_{51} + T_{54} < 0$ respectively; As for $\delta = 0$, we only need to adjust node no. 6 as a fixed point.

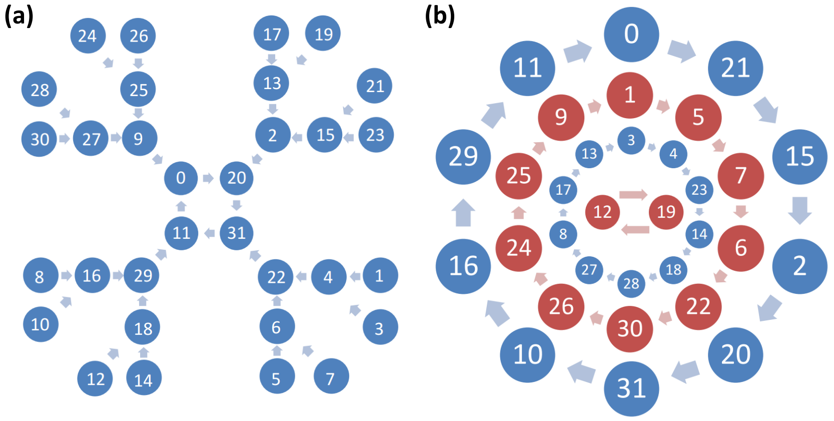


FIG. 2: Structures of the deterministic model when $T_{51} + T_{54} \neq 0$ with $\delta = 1$ in the case $T_{51} + T_{54} > 0$ (a) and $T_{51} + T_{54} < 0$ (b). As for $\delta = 0$, we only need to adjust node no. 6 as a fixed point.

Then, we assume in the following analysis that

$$T = \begin{pmatrix} 0 & 0 & 0 & 0 & -t_1 \\ t_2 & 0 & 0 & 0 & 0 \\ 0 & -t_3 & 0 & 0 & 0 \\ 0 & 0 & t_4 & 0 & 0 \\ t_5 & 0 & 0 & -t_5 & 0 \end{pmatrix},$$

where $t_i \in (0, 2],\ \forall i$.

According to our theory, we find out that when $\delta = 1$, all the key paths that possibly influence the minimum activation energy barrier from cycle 1 to cycle 2 are:

$$\begin{aligned} 9 \to 0, \quad 22 \to 31 &: \text{with activation energy barrier } k; \\ 1 \to 21, \quad 5 \to 23, \quad 26 \to 8, \quad 30 \to 10 &: \text{with activation energy barrier } 2t_1; \\ 5 \to 15, \quad 26 \to 16 &: \text{with activation energy barrier } 2t_2; \\ 7 \to 2, \quad 24 \to 29 &: \text{with activation energy barrier } 2t_3; \\ 6 \to 20, \quad 25 \to 11 &: \text{with activation energy barrier } 2t_4. \end{aligned}$$

Thus the minimum activation energy barrier from cycle 1 to cycle 2 equals $\min\{k, 2t_1, 2t_2, 2t_3, 2t_4\}$.

Similarly, all the key paths that possibly influence the minimum activation energy barrier from cycle 2 to cycle 1 are:

$$\begin{aligned} 0 \to 4, \quad 31 \to 27 &: \text{with activation energy barrier } 2t_1; \\ 0 \to 28, \quad 31 \to 3 &: \text{with activation energy barrier } 2t_2; \\ 11 \to 4, \quad 20 \to 27 &: \text{with activation energy barrier } 2t_3; \\ 0 \to 22, \quad 31 \to 9 &: \text{with activation energy barrier } 2t_4. \end{aligned}$$

Thus the minimum activation energy barrier from cycle 2 to cycle 1 equals $\min\{2t_1, 2t_2, 2t_3, 2t_4\}$.

Therefore, when $k < \min\{2t_1, 2t_2, 2t_3, 2t_4\}$, the minimum activation energy barrier from cycle 1 to cycle 2 is lower than that in the opposite direction, resulting in global attractive behavior of cycle 2(Phase I); otherwise the two minimum activation energy barriers are equal to each other, resulting a non-degenerate probability distribution between the two cycles (Phase II).

To be more specific, we now limit our discussion to how the model changes when each nonzero element of $T$ diverge slightly from their original values. If $k > 2$, we know from the above reasoning that with the original $T$, the model is not global attractive; Moreover, there are 10 optimal paths from cycle 1 to cycle 2 and 8 from cycle 2 to cycle 1 respectively. When $t_1$ increases slightly, the minimum activation energy barriers in both direction remain to be 2, while there are 6 optimal paths from cycle 1 to cycle 2 and 6 from cycle 2 to cycle 1 respectively. When $t_1$ decreases slightly, the minimum activation energy barriers in both direction becomes $t_1$, while there will be 4 optimal paths from cycle 1 to cycle 2 and 2 from cycle 2 to cycle 1 respectively. When $t_2$ increases slightly, the minimum activation energy barriers in both directions remains to be 2, while there are 8 optimal paths from cycle 1 to cycle 2 and 6 from cycle 2 to cycle 1 respectively. When $t_2$ decreases slightly, the minimum activation energy barriers in both directions becomes $t_2$, while there are 2 optimal paths from cycle 1 to cycle 2 and 2 from cycle 2 to cycle 1 respectively. The impact of $t_3$ and $t_4$ is similar to $t_2$, and changes in $t_5$ do not influence the model.

If $k = 2$, the model with the original $T$ is also not global attractive; Furthermore, there are 12 optimal paths from cycle 1 to cycle 2 and 8 from cycle 2 to cycle 1 respectively. When $t_1$ increases slightly, the minimum activation energy barriers in both directions remain to be 2, while there are 8 optimal paths from cycle 1 to cycle 2 and 6 from cycle 2 to cycle 1 respectively. When $t_1$ decreases slightly, the minimum activation energy barriers in both directions become $t_1$, while there are 4 optimal paths from cycle 1 to cycle 2 and 2 from cycle 2 to cycle 1 respectively. When $t_2$ increases slightly, the minimum activation energy barriers in both directions remain to be 2, while there are 10 optimal paths from cycle 1 to cycle 2 and 6 from cycle 2 to cycle 1 respectively. When $t_2$ decreases slightly, the minimum activation energy barriers in both directions become $t_2$, while there are 2 optimal paths from cycle 1 to cycle 2 and 2 from cycle 2 to cycle 1 respectively. The impact of $t_3$ and $t_4$ is similar to $t_2$, and changes in $t_5$ do not influence the model.

If $k < 2$, the model with the original $T$ shows global attractive behavior in cycle 2, which means that the minimum activation energy barrier from cycle 1 to cycle 2 is lower than that in the opposite direction. Apparently, this fact will not be changed with sufficient small changes in $t_j$ $(j = 1, ..., 5)$.

Combining the above information together, we could easily compute the probability distribution of cycle 1 (i.e. $P_1 = |A_1| \times c_1$), as well as the minimum activation energy barriers in both directions. Fig. 3 (a) presents the value of $P_1$ when we make adjustments under the case $\delta = 1$, $k = 2$, while Fig. 3 (b) shows how the minimum activation energy barriers change when each nonzero element of $T$ changed within $[0, 2]$ in this case. Fig. 3 (c) shows how the minimum activation energy barriers change

when each nonzero element of $T$ changed within $[0,2]$ under the case $\delta = 1$, $k < 2$. The case $\delta = 1$, $k > 2$ is illustrated in the main text.

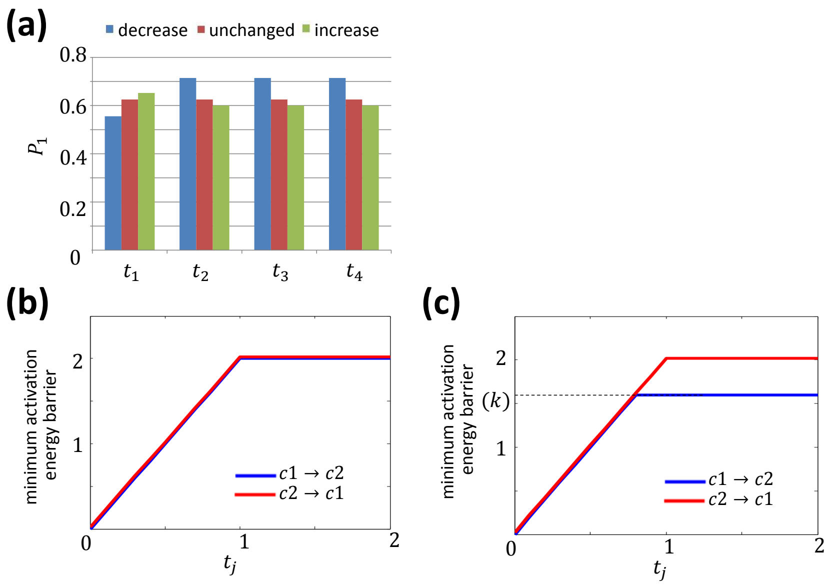


FIG. 3: Probability of cycle 1 (i.e. $P_1 = |A_1| \times c_1$) as well as the minimum activation energy barriers under slight changes in nonzero components of $T$. (a) $P_1$ as each nonzero component is increased (blue) or decreased (green) under the case $\delta = 1$, $k = 2$. The original $P_1$ is plotted in red for comparison. Note that $P_1$ remains to be 0 with small changes in all $t_j$'s under the case $\delta = 1, k < 2$. (b) Minimum activation energy barrier from cycle 1 to cycle 2 (blue) and that from cycle 2 to cycle 1 (red) when a nonzero component changes in $[0,2]$, under the case $\delta = 1$, $k = 2$. They completely overlap with each other. (c) Minimum activation energy barrier from cycle 1 to cycle 2 (blue) and that from cycle 2 to cycle 1 (red) when a nonzero component changes in $[0,2]$, under the case $\delta = 1$, $k < 2$. Note that the blue solid line overlaps partly with the red solid line. In plotting this figure we take $k = 1.6$.

Next, we proceed to analyze the case with $\delta = 0$. This time, all the key paths that possibly influence the minimum activation energy barrier from node no. 6 to cycle 2 are:

$$6 \rightarrow 2 : \text{with activation energy barrier } 2t_3;$$
$$6 \rightarrow 22 \rightarrow 31, \quad 6 \rightarrow 22 \rightarrow 30 \rightarrow 26 \rightarrow 24 \rightarrow 25 \rightarrow 9 \rightarrow 0 : \text{with activation energy barrier } k + l.$$

This means that the minimum activation energy barrier from node "6" to cycle 2 equals $\min\{2t_3, k + l\}$. Meanwhile, all the key paths that possibly influence the minimum activation energy barrier from cycle 2 to node "6" are:

$$0 \rightarrow 4, \quad 31 \rightarrow 27 : \text{with activation energy barrier } 2t_1;$$
$$0 \rightarrow 28, \quad 31 \rightarrow 3 : \text{with activation energy barrier } 2t_2;$$
$$11 \rightarrow 4, \quad 20 \rightarrow 27 : \text{with activation energy barrier } 2t_3;$$
$$0 \rightarrow 22, \quad 31 \rightarrow 9 : \text{with activation energy barrier } 2t_4.$$

Thus the minimum activation energy barrier from cycle 2 to node no. 6 still equals $\min\{2t_1, 2t_2, 2t_3, 2t_4\}$.

We study how the model changes when each nonzero element of $T$ diverge slightly from their original values. If $k + l > 2$, we know from the above reasoning that with the original $T$, the model is not global attractive; Moreover, there are 1 optimal path from node no. 6 to cycle 2 and 8 from cycle 2 to node no. 6 respectively. When $t_1$ increases slightly, the minimum activation energy barriers in both direction will remain to be 2, while there is 1 optimal path from node no. 6 to cycle 2 and 6 from cycle 2 to node no. 6 respectively. When $t_1$ decreases slightly, the minimum activation energy barrier from node no. 6 to cycle 2 remains to be 2, but that from cycle 2 to node no. 6 drops to $2t_1$, which means that node no. 6 will become global attractive. When $t_3$ increases slightly, the minimum activation energy barrier from cycle 2 to node no. 6 remain to be 2, but that from node no. 6 to cycle 2 rises to $2t_3$, and thus node no. 6 also becomes global attractive. When $t_3$ decreases slightly, the minimum activation energy barriers in both directions will be reduced to $2t_3$ indicating no global attractive behavior will occur, and there is 1 optimal path from node no. 6 to cycle 2 and 2 from cycle 2 to node no. 6 respectively. The impact of $t_2$ and $t_4$ is similar to $t_1$, and changes in $t_5$ do not influence the model.

If $k + l = 2$, the model with the original $T$ is also not global attractive; Further, there are 3 optimal paths from node no. 6 to cycle 2 and 8 from cycle 2 to node no. 6 respectively. When $t_1$ increases slightly, the minimum activation energy barriers in both direction remain to be 2, while there are 3 optimal paths from node no. 6 to cycle 2 and 6 from cycle 2 to node no. 6 respectively. When $t_1$ decreases slightly, the minimum activation energy barrier from node no. 6 to cycle 2 remains to be 2, but that from cycle 2 to node no. 6 drops to $2t_1$, which means that node no. 6 becomes global attractive. When $t_3$ increases slightly, the minimum activation energy barriers in both directions remain to be 2, while there are 2 optimal paths from node no. 6 to cycle 2 and 6 from cycle 2 to node no. 6 respectively. When $t_3$ decreases slightly, the minimum activation energy barriers in both directions are reduced to $2t_3$, while there is 1 optimal paths from node no. 6 to cycle 2 and 2 from cycle 2 to node no. 6 respectively. The impact of $t_2$ and $t_4$ is similar to $t_1$, and changes in $t_5$ do not influence the model.

If $k+l < 2$, the model with the original $T$ shows global attractive behavior in cycle 2, which means that the minimum activation energy barrier from node no. 6 to cycle 2 is lower than that in the opposite direction. Apparently, this fact will not be changed with sufficient small changes in $t_j$ ($j = 1, ..., 5$).

Similarly, we could compute the probability of node no. 6 (also denoted as $P_1$) as well as the minimum activation energy barriers in both directions. Fig. 4 (a) presents the values of $P_1$ at the condition $\delta = 0$, $k + l = 2$. Fig. 4 (b) depicts the variation of the minimum activation energy barriers as a function of $t_j$ at $\delta = 0, k + l = 2$, whereas, the same quantity has been plotted in Fig. 4 (c) as a function of $t_j$ at different condition where $\delta = 0, k + l < 2$. The case $\delta = 0$, $k + l > 2$ has been illustrated in the main text.

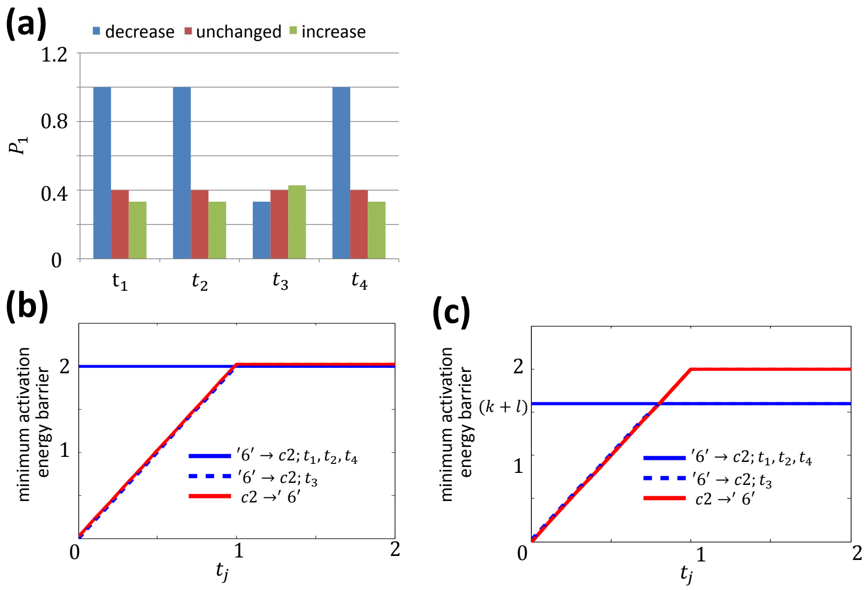


FIG. 4: Probability of node "6" (i.e. $P_1 = |A_1| \times c_1$) as well as the minimum activation energy barriers under slight changes in nonzero components of $T$. (a) $P_1$ as each nonzero component is increased (blue) or decreased (green) under the case $\delta = 0$, $k + l = 2$. The original $P_1$ is plotted in red for comparison. Note that $P_1$ remains to be 0 with small changes in all $t_j$'s under the case $\delta = 0, k + l < 2$. (b)Minimum activation energy barrier from node "6" to cycle 2 (blue) and that from cycle 2 to node "6" (red) when each nonzero component of $T$ changes in $[0, 2]$, under the case $\delta = 0$, $k + l = 2$. Note that the red solid line and the blue dashed line overlap entirely. (c) Minimum activation energy barrier from node "6" to cycle 2 (blue) and that from cycle 2 to node "6" (red) when each nonzero component of $T$ changes in $[0, 2]$, under the case $\delta = 0$, $k + l < 2$. Note that the red solid line overlaps partly with the blue dashed line. In plotting this figure we take $k + l = 1.6$.

* Electronic address: haoge@pku.edu.cn

[1] Chen, D., Feng, J. and Qian M. (1994) *Science in China* **39**, 7-28.
